# Supplementary material for: Cross-Dataset Linkage of Brain MRI using Image Similarity Measures
Source: arXiv:2602.10043 source file (2026-05-05)
Supplement: Supplementary file 1 [file Supplementary_Information.pdf]

# Simple Image Processing and Similarity Measures Can Link Data Samples across Databases through Brain MRI

**Gaurang Sharma, Harri Pölönen, Juha Pajula, Jutta Suksi, and Jussi Tohka, for the Alzheimer’s Disease Neuroimaging Initiative**

## Results

This section contains the pre-evaluation and evaluation results on the selected datasets.

**Simulated Human Connectome Project (SHCP):** Dataset formed by perturbing 100 random images from the HCP Young Adult Dataset, leading to 500 images. Pre-evaluation results are present in the Supplementary Information Figure 1 and their quantitative results are presented in the Supplementary Information Supplementary Information Table 1.

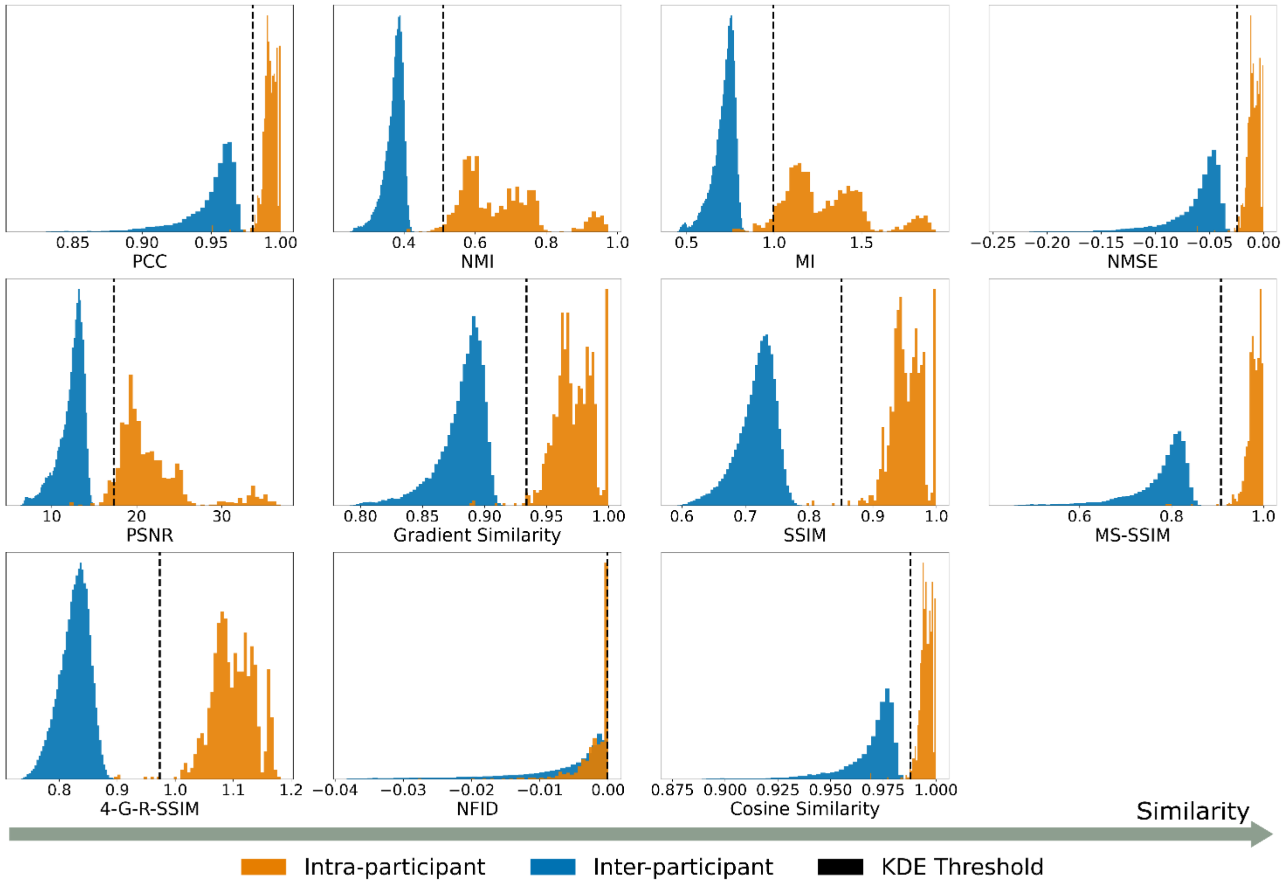


*Supplementary Information Figure 1: Pre-evaluation results on SHCP indicated that, following harmonization, all similarity measures except FID clearly separated inter- and intra-participant distributions, albeit with minor overlap. For visualization, high-FID outliers were removed (12345 negative FID values < - 0.3568) using the interquartile range (IQR) method.*

The quantitative results are presented in the Supplementary Information Table 1.

*Supplementary Information Table 1: Pre-evaluation quantitative results on the SHCP dataset, providing the details of the Supplementary Information Figure 1.*

| Metric | KDE Threshold | AUC | Sensitivity | Specificity | Overlap |
|---|---|---|---|---|---|
| **PCC** | 0.9800 | 0.9979 | 0.9900 | 1.0000 | 0.0042 |
| **NMI** | 0.5104 | 0.9999 | 0.9830 | 1.0000 | 0.0030 |
| **MI** | 0.9956 | 0.9994 | 0.9510 | 1.0000 | 0.0077 |
| **NMSE** | 0.0245 | 0.9978 | 0.9900 | 1.0000 | 0.0054 |
| **PSNR** | 17.3369 | 0.9978 | 0.9430 | 1.0000 | 0.0047 |
| **Gradient Similarity** | 0.9338 | 0.9989 | 0.9920 | 1.0000 | 0.0042 |
| **SSIM** | 0.8510 | 1.0000 | 0.9960 | 1.0000 | 0.0000 |
| **MS-SSIM** | 0.9073 | 0.9984 | 0.9950 | 1.0000 | 0.0040 |
| **4-G-R-SSIM** | 0.9733 | 1.0000 | 0.9940 | 1.0000 | 0.0002 |
| **NFID** | 0.0001 | 0.8008 | 0.2600 | 1.0000 | 0.5679 |
| **Cosine Similarity** | 0.9878 | 0.9978 | 0.9870 | 1.0000 | 0.0054 |

**Simulated Latent Diffusion Model (SLDM):** Dataset formed by perturbing 100 random images from the LDM100K dataset, leading to 500 images. Pre-evaluation results are present in the main article, and the quantitative results are presented in the Supplementary Information Supplementary Information Table 2.

*Supplementary Information Table 2: Pre-evaluation quantitative results on the SLDM dataset, providing details of Figure 4 of the main article.*

| Metric | KDE Threshold | AUC | Sensitivity | Specificity | Overlap |
|---|---|---|---|---|---|
| **PCC** | 0.9680 | 1.0000 | 0.9950 | 1.0000 | 0.0001 |
| **NMI** | 0.4784 | 1.0000 | 0.9840 | 1.0000 | 0.0000 |
| **MI** | 0.8678 | 1.0000 | 0.9620 | 1.0000 | 0.0000 |
| **NMSE** | 0.0362 | 1.0000 | 0.9950 | 1.0000 | 0.0002 |
| **PSNR** | 15.2181 | 1.0000 | 0.9740 | 1.0000 | 0.0001 |
| **Gradient Similarity** | 0.9169 | 0.9998 | 0.9400 | 1.0000 | 0.0000 |
| **SSIM** | 0.8271 | 1.0000 | 1.0000 | 1.0000 | 0.0000 |
| **MS-SSIM** | 0.8602 | 1.0000 | 0.9990 | 1.0000 | 0.0000 |
| **4-G-R-SSIM** | 0.9645 | 1.0000 | 0.9950 | 1.0000 | 0.0000 |
| **NFID** | 0.0003 | 0.7493 | 0.1370 | 1.0000 | 0.5347 |
| **Cosine Similarity** | 0.9792 | 1.0000 | 0.9960 | 1.0000 | 0.0002 |

**Hormonal Health Study (HHS) Dataset:**
Longitudinal Study

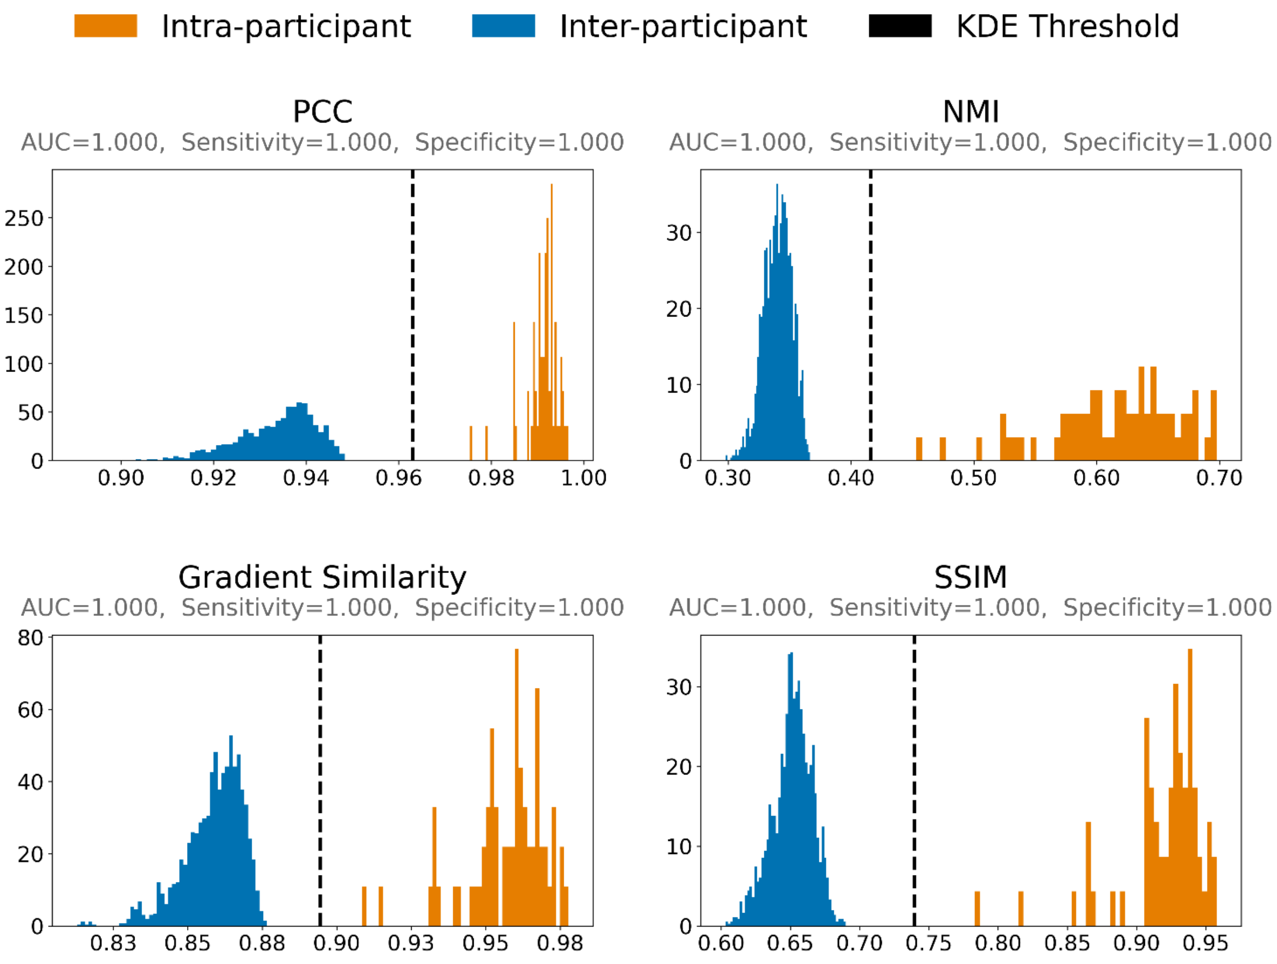


*Supplementary Information Figure 2: Evaluation results on the Hormonal Health Study. All measures showed clear divergence in the ground-truth–labeled density histograms.*

**Running Intervention Dataset:**
Longitudinal Study

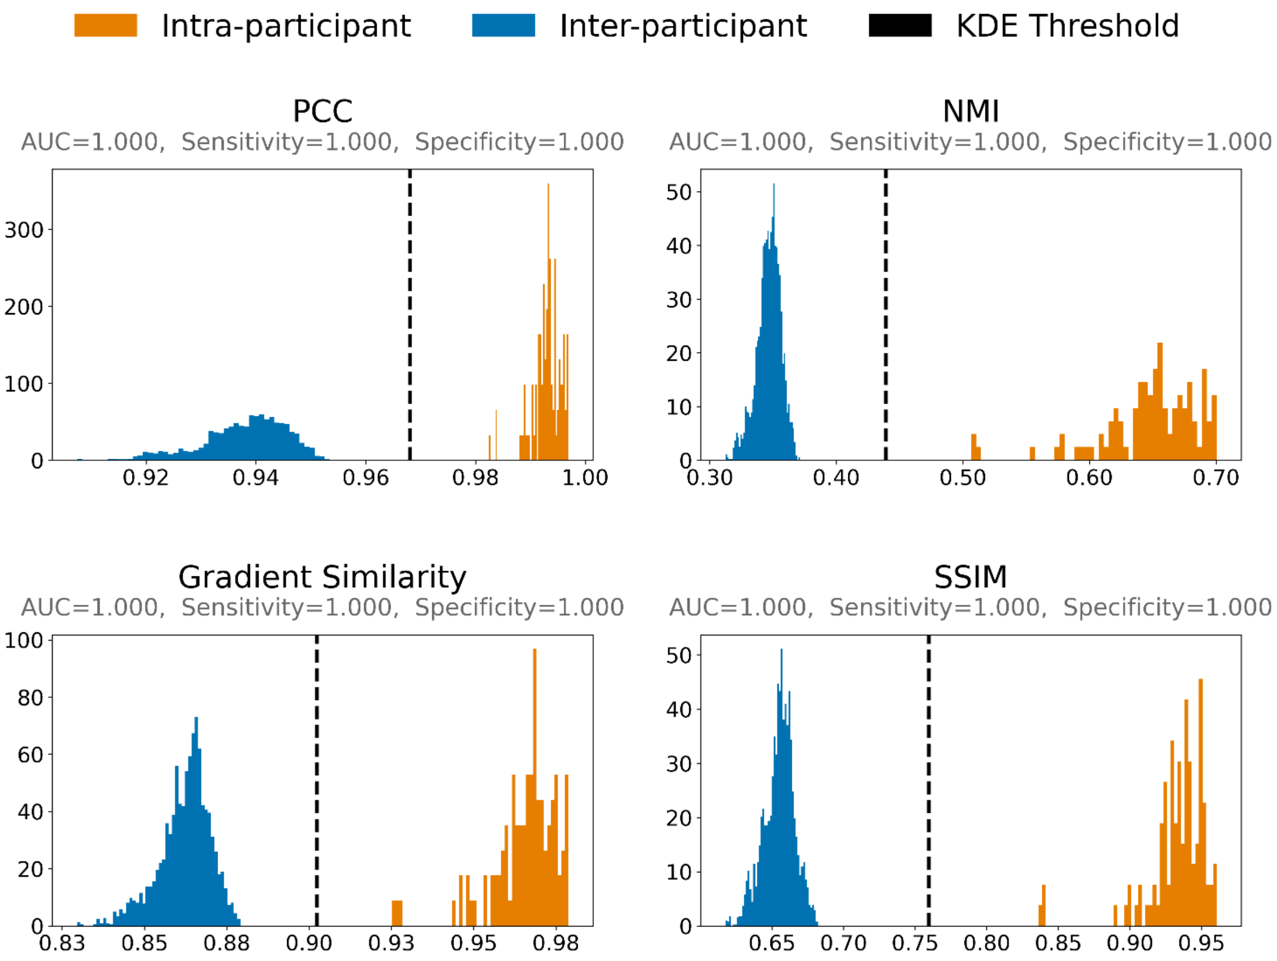


*Supplementary Information Figure 3: Evaluation results of running the intervention study. All measures showed clear divergence in the ground-truth–labeled density histograms.*

**Traveling Human Phantom (THP) Dataset**
Traveling Participant Study

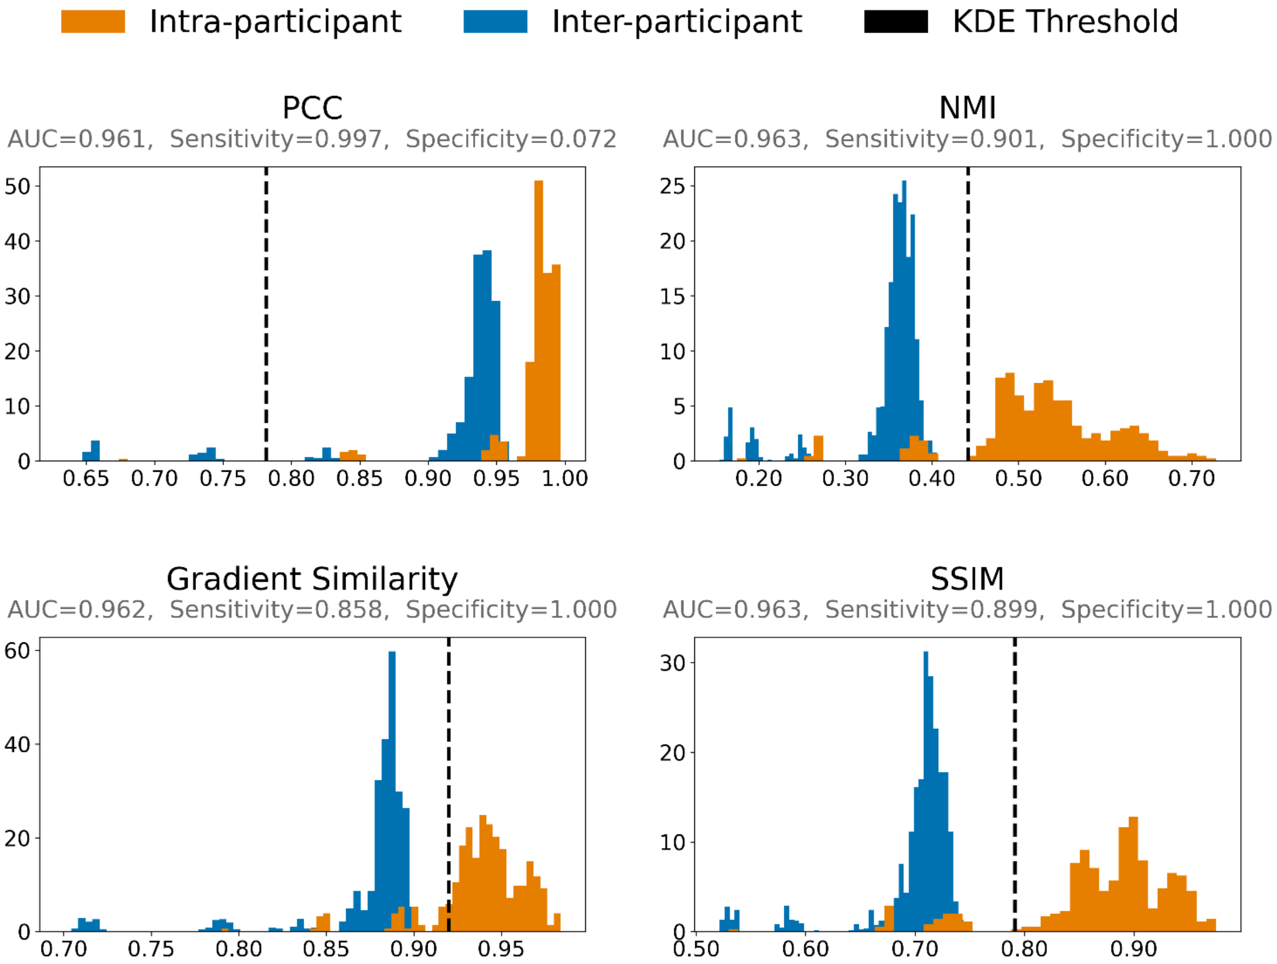


*Supplementary Information Figure 4: Evaluation results on the traveling participant-based study on the THP datasets demonstrate strong performance across measures, with perfect results in SSIM, NMI, and Gradient Similarity using the estimated thresholds. However, thresholding for PCC was unsuccessful due to outliers caused by poor image quality and the limited number of available images.*

**San Diego State University Traveling Participants Dataset (SDSU-TS)**
Travelling Participant Study

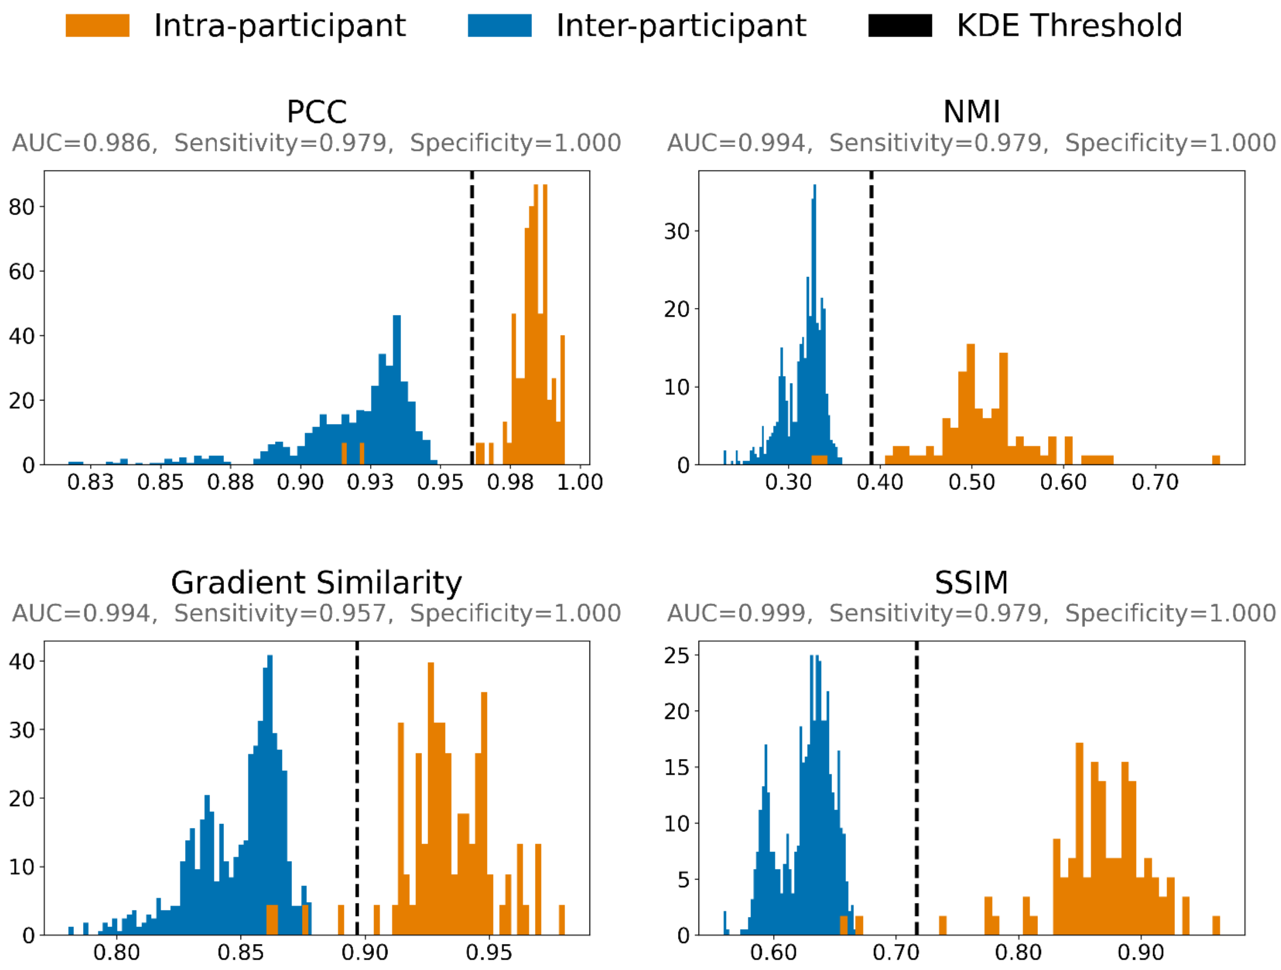


*Supplementary Information Figure 5: Evaluation results on a traveling participant-based study on the SDSU-TS dataset, showing near-perfect performance on similarity measures.*

**ADNI Dataset:**

This section shows two images per participant acquired under the ADNI1 and ADNI2 protocols (IDs 378 and 915). Participant 378 progressed to dementia, while 915 continued with the cognitive status with an existing dementia diagnosis. These examples confirm that participant matching remains feasible despite changes in cognitive status, time interval, and imaging protocol.

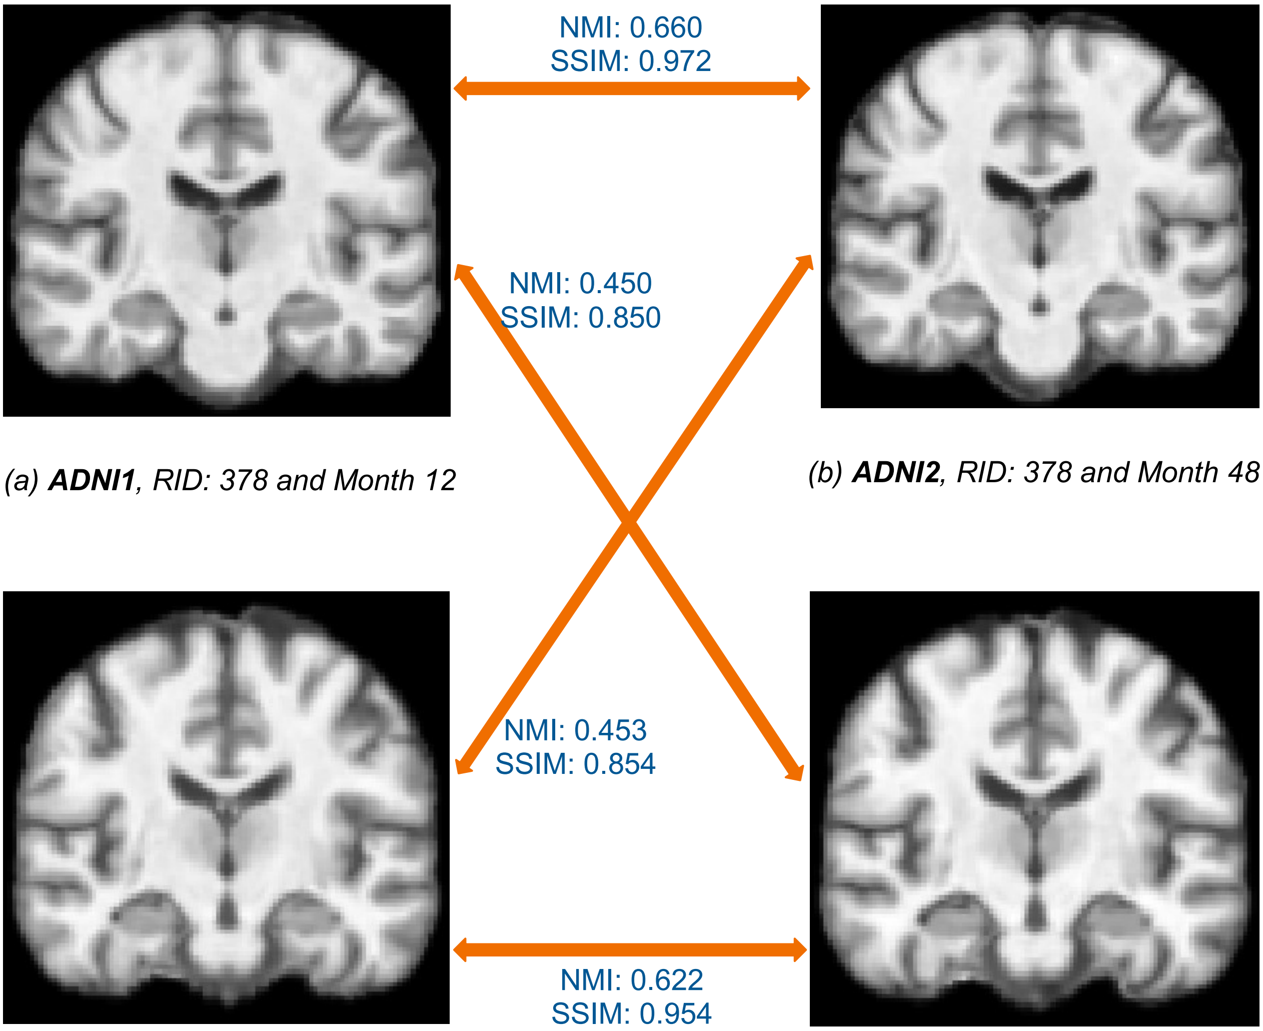


*(a)* ***ADNI1****, RID: 378 and Month 12*

*(b)* ***ADNI2****, RID: 378 and Month 48*

*(c)* ***ADNI1****, RID: 915 and Month 18*

*(d)* ***ADNI2****, RID: 915 and Month 66*

*Supplementary Information Figure 6: Evaluation results on the ADNI dataset: participant matching remains feasible despite changes in cognitive status, time interval, and imaging protocol. The left column shows MRIs acquired under the ADNI1 protocol, and the right column shows MRIs acquired under the ADNI2 protocol, with an MNI y-coordinate of -18mm. Participant RID 378 progressed from MCI to dementia, yet the similarity between the two scans remained high (SSIM = 0.972, NMI = 0.660), exceeding the thresholds (SSIM = 0.885, NMI = 0.517). Participant RID 915, already diagnosed with dementia, likewise exhibited high similarity (SSIM = 0.954, NMI = 0.622). In contrast, inter-participant comparisons yielded similarity scores below the thresholds (example, SSIM = 0.850 and NMI = 0.450). These patterns occurred irrespective of structural changes associated with dementia progression or continuation over 36 months for RID 378 and 48 months for RID 915.*

**Data**

This section lists the participant IDs whose T1w MRI scans were used for the pre-evaluation datasets (SLDM and SHCP) and for the evaluation of the ADNI dataset. For all other datasets, all available scans from a were included.

**SLDM**

065510 069497 059367 033916 037592 074207 014612 061005 003574 077143 068061 064169 004274 028568 055152 065969 091284 081821 089042 097292 023859 033071 081267 016423 042614 072239 057686 035648 065763 019591 034352 074159 058884 025860 017316 031550 034391 012457 031429 075692 077067 012768 044854 006866 073221 076040 038085 060104 052599 006309 079695 072520 067502 051641 025996 033015 085593 072619 059751 083212 085425 009561 012605 080513 035982 014141 087837 043204 014256 009361 041521 026410 032471 080140 042554 069966 037353 088367 058343 052798 062754 054551 055429 092549 080649 077322 064362 069973 017383 063429 036486 008293 062742 045376 053438 039910 088291 020172 001610 029555

**SHCP**

100408 101410 104012 113215 113619 114318 114419 117324 118831 123723 130518 133928 134324 135225 137128 137431 137936 138231 138332 139637 140420 144226 146331 148436 148941 149539 153833 153934 156637 158136 159239 163331 163836 165234 165840 167238 168947 177746 182436 183337 185139 186444 191033 196952 199150 199958 200109 201414 203721 204218 205220 205725 205826 207426 208024 208630 209228 211417 334635 336841 339847 346137 355845 360030 366042 379657 392750 393247 395251 397861 432332 475855 495255 553344 567052 580650 587664 626648 663755 672756 680250 688569 689470 737960 753251 788674 792766 803240 804646 825048 825654 837964 844961 859671 878877 885975 894673 901442 930449 953764

**ADNI**

21 23 31 42 51 55 56 58 59 61 69 72 74 89 96 101 106 107 108 112 113 116 120 123 126 127 130 135 142 150 156 159 160 166 169 171 172 173 186 200 210 214 217 225 227 229 230 232 257 259 260 269 272 276 285 289 291 292 295 296 298 301 303 307 311 315 331 337 352 359 361 376 377 378 382 384 408 413 416 419 420 441 454 467 473 479 498 501 505 514 519 520 522 545 546 548 552 553 555 563 566 588 602 605 610 618 626 644 658 667 668 671 677 679 680 685 698 702 709 717 722 729 731 734 741 746 751 752 767 778 800 802 824 830 835 842 863 867 872 886 887 896 906 907 908 914 915 919 920 922 923 925 926 934 951 952 969 972 984 985 989 994 997 1004 1016 1023 1030 1032 1034 1043 1045 1046 1052 1057 1066 1072 1074 1078 1097 1098 1106 1117 1118 1122 1123 1130 1148 1155 1169 1186 1187 1190 1195 1202 1203 1206 1222 1232 1242 1243 1246 1249 1250 1255 1256 1261 1268 1271 1280 1286 1288 1300 1318 1326 1331 1346 1351 1352 1378 1380 1394 1407 1408 1414 1419 1425 1427
